# Supplementary material for: Continuous Time Frank-Wolfe Does Not Zig-Zag, But Multistep Methods Do Not Accelerate
Source: arXiv:2106.05753 source file (2022-02-01)
Supplement: Supplementary file 1 [file supplementary.tex]

%%%%%%%% ICML 2022 EXAMPLE LATEX SUBMISSION FILE %%%%%%%%%%%%%%%%%

\documentclass[nohyperref]{article}

% Recommended, but optional, packages for figures and better typesetting:
\usepackage{microtype}
\usepackage{graphicx}
\usepackage{subfigure}
\usepackage{booktabs} % for professional tables

% hyperref makes hyperlinks in the resulting PDF.
% If your build breaks (sometimes temporarily if a hyperlink spans a page)
% please comment out the following usepackage line and replace
% \usepackage{icml2022} with \usepackage[nohyperref]{icml2022} above.
\usepackage{hyperref}

% Attempt to make hyperref and algorithmic work together better:

% Use the following line for the initial blind version submitted for review:
\usepackage{icml2022}

% If accepted, instead use the following line for the camera-ready submission:
% \usepackage[accepted]{icml2022}

% For theorems and such
\usepackage{amsmath}
\usepackage{amssymb}
\usepackage{mathtools}
\usepackage{amsthm}

%%added packages
\usepackage{caption}
\usepackage{enumitem}
\usepackage{multirow}

%% macros here

%\newcommand{\lmoref}{\textrm{(LMO)}}

\newcommand{\bmat}{\begin{bmatrix}}
\newcommand{\emat}{\end{bmatrix}}

%%macros for editing, remove before submission
%\newcommand{\red}[1]{{\color{red}#1}}
%\newcommand{\blue}[1]{{\color{blue}#1}}
%\newcommand{\gray}[1]{{\color{gray}#1}}
%\newcommand{\green}[1]{{\color{teal}#1}}

% if you use cleveref..
\usepackage[capitalize,noabbrev]{cleveref}

%%%%%%%%%%%%%%%%%%%%%%%%%%%%%%%%
% THEOREMS
%%%%%%%%%%%%%%%%%%%%%%%%%%%%%%%%
\theoremstyle{plain}

\theoremstyle{definition}

\theoremstyle{remark}

% Todonotes is useful during development; simply uncomment the next line
%    and comment out the line below the next line to turn off comments
%\usepackage[disable,textsize=tiny]{todonotes}
\usepackage[textsize=tiny]{todonotes}

% The \icmltitle you define below is probably too long as a header.
% Therefore, a short form for the running title is supplied here:
\icmltitlerunning{Continuous Time FW Does Not Zig-Zag,
But Multistep Methods Do Not Accelerate}

\begin{document}

\bibliographystyle{icml2022}

\newpage
\appendix
\onecolumn
\input{sections/appendix}

\end{document}
